# Supplementary material for: Scaling study of diffusion in dynamic crowded spaces
Source: arXiv:2011.02444 source file (2024-10-09)
Supplement: Supplementary file 1 [file SI.pdf]

# Supplementary Material for “Scaling study of diffusion in dynamic crowded spaces”

H. Bendekgey,<sup>1,2</sup> G. Huber,<sup>1</sup> and D. Yllanes<sup>1,3,\*</sup>

<sup>1</sup>Chan Zuckerberg Biohub, San Francisco, California 94158, USA

<sup>2</sup>University of California, Irvine, California 92697, USA

<sup>3</sup>Instituto de Biocomputación y Física de Sistemas Complejos (BIFI), 50009 Zaragoza, Spain

(Dated: November 3, 2020)

## Finite-Size Effects

Our model does not suffer from strong finite-size effects, probably thanks to the annealed nature of the disorder. Therefore, our simulations for  $L = 1000$  should be representative of the large- $L$  limit. We have, nevertheless, explicitly checked against finite-size effects by repeating our  $\hat{n} = \hat{n}_c$  simulations for a smaller system size ( $L = 500$ ) and verifying that we get the same  $D(t)$  curve as in Figure 2 in the paper. This is shown in Figure S1. For all  $D_{\text{obs}}$  the resulting  $D_{\text{eff}}$  is the same in the  $L = 500$  system, but the data is noisier.

## Time evolution in the sub- and supercritical regimes

Figure 2 in the paper shows  $D(t)$  for many obstacle diffusivities at  $\hat{n} \approx \hat{n}_c$ . In Figures S2 and S3 we reproduce the same plot for a subcritical density ( $\hat{n} = 0.2$ ) and a supercritical one ( $\hat{n} = 0.4$ ). The resulting plots are qualitatively the same as Figure 2. Notice in particular that, even in the supercritical case, above the percolation point, the diffusive regime is eventually reached.

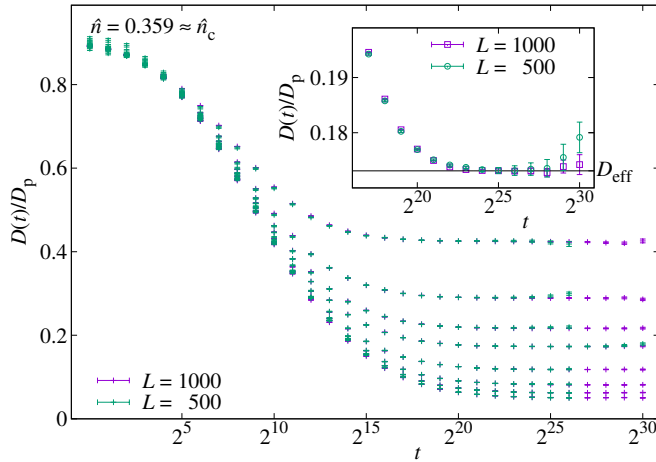

FIG. S1. Same as Figure 2 in the paper, but adding data for a smaller system size ( $L = 500$ ). Since the curves for  $L = 1000$  and  $L = 500$  are identical for the whole  $t$  range, we have only plotted most of the small simulations up to  $t = 2^{26}$  for visualization purposes. The exception is  $D_{\text{obs}}/D_p = 10^{-2.4}$ , enlarged in the inset. The  $L = 500$  curve are noisier for long  $t$  where there are few  $t_0$  to compute the MSD.

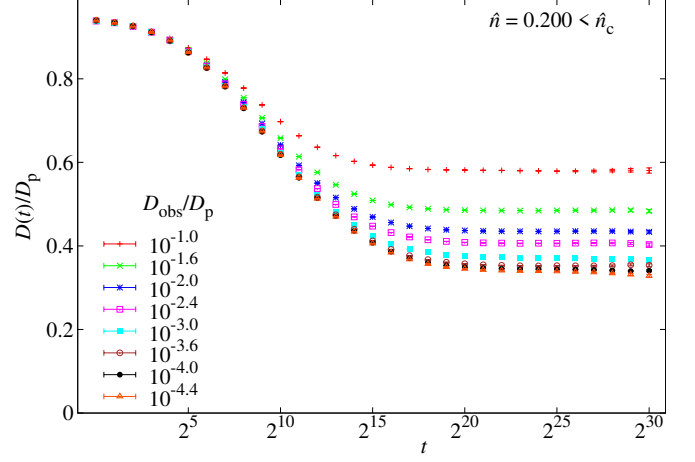

FIG. S2. Same as Figure 2 in the paper, but for a subcritical obstacle concentration ( $\hat{n} = 0.2$ ).

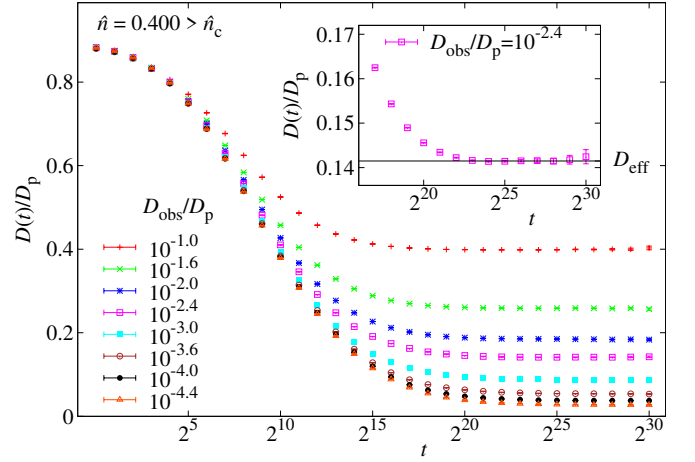

FIG. S3. Same as Figure 2 in the paper, but for a supercritical obstacle concentration ( $\hat{n} = 0.4$ ). The inset shows that the long-time diffusive regime [constant  $D(t)$ ] is clearly reached.

## Unscaled $D_{\text{eff}}$ in $d = 3$

The time-dependent diffusion coefficient  $D(t)$  and the effective diffusivity  $D_{\text{eff}}$  have qualitatively the same behavior in  $d = 3$  as in  $d = 2$ , but  $D_{\text{eff}}$  is governed by different scaling exponents as shown in Figure 5. In Figure S4 we plot the unscaled  $D_{\text{eff}}$  for all our  $d = 3$  simulations.

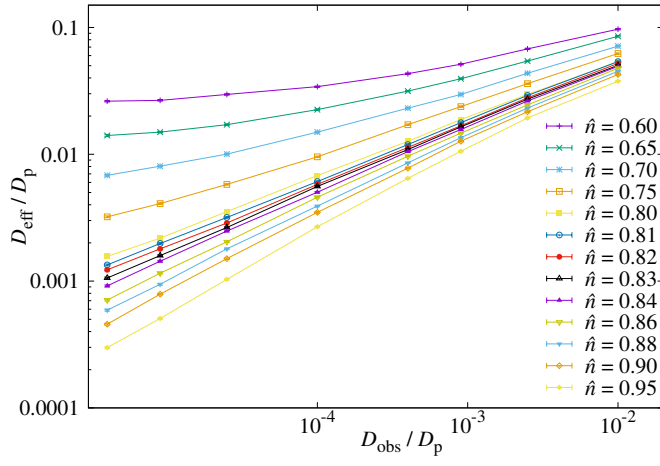

FIG. S4. Effective diffusion coefficient against the diffusion coefficient of the obstacles for many obstacle densities in  $d = 3$ . The percolation density is  $\hat{n}_c \approx 0.839$ .
